# Supplementary material for: Localized Uncertainty Attacks
Source: arXiv:2106.09222 source file (2021-06-17)
Supplement: Supplementary file 1 [file appendix.tex]

\onecolumn
\appendix
\section{Background on Manifold Learning} ~\label{app:background}
Our proposed attack uses manifold learning to first map the inputs to a low-dimensional embedding space and then uses this embedding space representation to craft an adversarial example. Manifold learning is based on the assumption that high dimensional data lies on or near lower dimensional manifolds in a latent space. Our paper uses a Variational Auto-Encoder (VAE) trained using Stein Variation Gradient Descent (SVGD) for manifold learning. We provide background information on VAEs and SVGD in this section before describing our attack framework in section~\ref{sec:framework}.

%One way to learn the manifold is by using VAEs. However, due to assumptions about the prior, VAEs can result in uninformative latent codes. In this section, we provide background on VAEs and then describe our proposed manifold learning technique using SVGD, which avoids the issues faced by VAEs.
 
 \subsection{Variational Auto Encoders}\label{sec:vae}
 VAEs~\cite{kingma2014} model the datapoints $x_n\in\mathcal{D}$ using a decoder $x_n \sim p(x_n|z_n; \phi)$. To learn $\phi$, one typically maximizes a variational approximation to the empirical  expected log-likelihood $1/N\sum_{n=1}^N \log p(x_n; \phi)$, called evidence lower bound (ELBO), defined as:
\begin{equation*}
    \begin{split}
     \mathcal{L}_\text{e}(\phi, \psi; x) &= \E_{q(z|x; \psi)}\log \left[\frac{p(x|z; \phi)p(z)}{q(z|x; \psi)} \right] \\
     &= - \mathbb{KL}(q(z|x; \psi)\|p(z|x; \phi)) + \log p(x; \phi).
     \label{eq:elbo}
    \end{split}  
\end{equation*}
Here, $q(z|x;\psi)$ denotes the encoder function. The expectation $\E_{q(z|x; \psi)}$ can be re-expressed as a sum of a reconstruction loss, or expected negative log-likelihood of $x$, and $\mathbb{KL}(q(z|x; )\|p(z))$. The $\mathbb{KL}$ forces the encoder $q_{\psi}$ to follow a distribution similar to $p(z)$. VAEs learn an encoding function that maps the data manifold to an isotropic Gaussian. However, \cite{2015arXiv150505770J} have shown that the Gaussian form imposed on $p(z)$ may result in uninformative latent codes; \textit{hence to poorly learning the semantics of} $\mathcal{D}$~\cite{DBLP:journals/corr/ZhaoSE17b}. 
To sidestep this issue, we minimize the divergence $\mathbb{KL}(q(z|x; \psi)\|p(z|x; \phi))$ using Stein Variational Gradient Descent~\cite{qiangliu2016} instead of explicitly optimizing the ELBO.

\subsection{Stein Variational Gradient Descent} 
SVGD is a nonparametric variational inference method that combines the advantages of MCMC sampling and variational inference. Unlike ELBO~\cite{kingma2014}, SVGD does not confine a target distribution $p(z)$ it approximates to simple or tractable parametric distributions. It remains an efficient algorithm. To approximate $p(z)$, SVGD maintains $M$ particles $\mathbf{z} = \{z_i\}_{i=1}^M$, initially sampled from a simple distribution, it iteratively transports via functional gradient descent. 
At iteration $t$, each particle $z^t\in \mathbf{z}^t$ is updated as:  
\begin{equation}
    \begin{gathered}
        z^{t+1} \leftarrow z^{t} + \alpha^{t}\tau(z^t)\ \text{where}\\
        \begin{aligned}
            \tau(z^t) = \frac{1}{M}\sum_{i=1}^M \Big[& k(z^t_i, z^t) \nabla_{z^t_i} \log p(z^t_i) + \nabla_{z^t_i} k(z^t_i, z^t) \Big],
        \end{aligned}
    \end{gathered}
    \label{eq:svgd}
\end{equation}
where $\alpha_t$ is a step-size and $k(., .)$ is a positive-definite kernel. In Equation~\ref{eq:svgd}, each particle determines its update direction by consulting with other particles and asking their gradients. The importance of the latter particles is weighted according to the distance measure $k(.,.)$. Closer particles are given higher consideration than those lying further away. The term $\nabla_{z_i}k(z_i, z)$ is a regularizer that acts as a repulsive force between the particles to prevent them from collapsing into one particle. Upon convergence, the particles $z_m$ will be unbiased samples of the true distribution $p(z)$.

\clearpage
\section{Algorithms for Our Proposed Attack} ~\label{app:algorithm}

\begin{figure*}[h]
\begin{minipage}[h]{0.48\textwidth}
    \includegraphics[width=8.0cm]{figures/inversion.png}
\end{minipage}
\begin{minipage}{0.48\textwidth}
\begin{algorithm}[H]
\begin{algorithmic}[1]
   \Require{Input $x\in\boldsymbol{\mathcal{D}}$}
   \Require{Model parameters $\boldsymbol{\eta}$}
   \State{Sample $\boldsymbol{\xi}\sim \mathcal{N}(\mathbf{0, I})$}
   \State{Get the weight vector $\boldsymbol{\theta} = \boldsymbol{f_{\eta}}(\boldsymbol{\xi})$}
   \State{Given $x$, sample $z\sim p(z|x; \boldsymbol{\theta})$}
   \State{Sample $\tilde{x}\sim p(x|z, \boldsymbol{\phi})$}
   \State{Sample $\tilde{z}\sim p(z|\tilde{x}, \boldsymbol{\theta})$}
   \State{Use $x$ and $\tilde{z}$ to compute $p(\tilde{z}|x; \boldsymbol{\theta})$}
\end{algorithmic}
   \caption{Inversion with one particle $\boldsymbol{\theta}$.}
   \label{alg:inversion}
\end{algorithm}
\end{minipage}
\caption{As the decoder $p_{\phi}$ gets more accurate (reconstruction loss $\|x - \tilde{x}\|_2$ becomes small), we get closer to the optimal $\tilde{z}$.}
\label{fig:invert}
\end{figure*}

\begin{algorithm*}[h]
   \caption{\textit{Adversarial Examples}. Lines 7 computes distances between sets keeping a one-to-one mapping.}
   \label{alg:algo_training}
\begin{algorithmic}[1]
   \Require{Training samples $(x, y)\in\boldsymbol{\mathcal{D}}\times\boldsymbol{\mathcal{Y}}$}
   \Require{Number of model instances $M$ and inner updates $T$}
   \Require{Initialize weights $\boldsymbol{\eta, \phi}$}\Comment{recognition net $f_{\eta}$, decoder $p_\phi$}
  \Require{Learning rates $\boldsymbol{\alpha, \beta}$}
   \State{Sample $\boldsymbol{\xi_1, ..., \xi_M}$ from $\mathcal{N}(\mathbf{0, I})$} \Comment{inputs to recognition net $f_{\eta}$}
   \For{$t=1$ {\bfseries to} $T$}
        \State{Sample $\boldsymbol{\Theta}=\{\boldsymbol{\theta_m}\}^M_{m=1}$ where $\boldsymbol{\theta_m} = \boldsymbol{f_{\eta}}(\boldsymbol{\xi_m})$}
        \State{Sample $z_1, ..., z_M$ using $\boldsymbol{\Theta}$} in Equation~\ref{eq:task_pos}
        %\If{$n > 1$}
        \State{Using Equation~\ref{eq:noise_inj}, get $z'_1, .., z'_M$} and average them to get $z'$ \Comment{learn latent perturbations $\delta_1, ..., \delta_M$}
        \State{Sample $\tilde{x}\sim p(x|z, \boldsymbol{\phi})$ and $x'\sim p(x'|z', \boldsymbol{\phi})$} \Comment{clean and perturbed reconstructions}
        \State{$\boldsymbol{\eta}\leftarrow \boldsymbol{\eta} - \boldsymbol{\alpha}\nabla_{\boldsymbol{\eta}} \|\boldsymbol{\Theta}\, - \texttt{\textbf{SVGD}}_{\tau}(\boldsymbol{\Theta})\|_2 $} (requires $\tilde{x}$) \Comment{apply \textit{inversion} on $\tilde{x}$ and update $\eta$}
        %\EndIf
   \EndFor
   \State{$\boldsymbol{\mathcal{L}}_{\tilde{x}}\coloneqq \|x - \tilde{x}\|_2; \hspace{.3cm} \boldsymbol{\mathcal{L}}_{x'}\coloneqq -\min\limits_{y'\in\mathcal{Y}\setminus\{y\}}\log\left(P(y'|x'; \nu)\right) + \lambda * \|x-x'\|_2$}\Comment{scaling reconstruction loss on $x' \text{ by }\lambda$}
   \State{$\boldsymbol{\phi}\leftarrow \boldsymbol{\phi} - \boldsymbol{\beta}\nabla_{\boldsymbol{\phi}}(\boldsymbol{\mathcal{L}}_{\tilde{x}} + \boldsymbol{\mathcal{L}}_{x'})$}\Comment{decoder update using Adam optimizer}
\end{algorithmic}
\end{algorithm*}

\section{Additional Experiments}~\label{app:additional_experiments}

\subsection{Manifold Preservation}~\label{app:swiss_roll}
We experiment with a 3D non-linear Swiss Roll dataset comprising of 1600 datapoints grouped in 4 classes. Figure~\ref{fig:swissroll} shows the 2D plots of the latent codes from the learnt manifold (left), latent codes of adversarial examples (with $\epsilon_\text{attack}\leq 0.3$) produced by our attack (center) and latent codes of PGD adversarial examples (right). These plots show that, unlike PGD, the latent codes of our adversarial examples are well-aligned with the manifold.

\begin{figure}[tbh]
\begin{center}
    \includegraphics[width=8.2cm]{samples/scatter-adv-all.pdf}
\end{center}
\caption{Swiss Roll manifold learned with encoder $E$ (left), and after  perturbing its elements with GBSM (middle) vs. that of PGD adversarial examples (right) learned using $E$.} 
	\label{fig:swissroll}
\vskip -.2in
\end{figure}

\subsection{Evaluations on Text Classification Task using SNLI Dataset}~\label{app:snli_exp}

We consider the SNLI~\cite{DBLP:journals/corr/BowmanAPM15} dataset. SNLI consists of sentence pairs where each pair contains a premise (\textit{P}) and a hypothesis (\textit{H}), and a label indicating the relationship (\textit{entailment, neutral, contradiction}) between the premise and hypothesis. For instance, the following pair is assigned the label \textit{entailment} to indicate that the premise entails the hypothesis.\\
\textit{Premise: A soccer game with multiple males playing. }
\textit{Hypothesis: Some men are playing a sport.}
\vspace{0.3em}

\noindent\textbf{Setup.} We perturb the hypotheses while keeping the premises unchanged. Similar to \cite{zhao2018generating}, we generate adversarial text at word level using a vocabulary of 11,000 words. We also use ARAE~\cite{pmlr-v80-zhao18b} for word embedding, and a CNN for sentence embedding. To generate perturbed hypotheses, we consider three types of decoders $p_\phi$: (i.)  a transpose CNN, (ii.) a language model, and (iii.) we use the decoder of a pre-trained ARAE model. The transpose CNN generates more meaningful hypotheses (see examples in  Table~\ref{tab:snli_results_appendix}) than the language model and the pre-trained ARAE model although we notice sometimes changes in the meaning of the original hypotheses. We discuss these limitations in Appendix where we provide also more examples of adversarial text.  

\ignore{
\begin{table}[ht]
\caption{Test samples and their perturbed versions.}
\label{tab:snli_results}
%\vskip -0.5in
%\begin{center}
\begin{small}
\begin{sc}
    \begin{tabular}{
        >{\arraybackslash}m{1.7cm}
        >{\arraybackslash}m{5.8cm}}
    \toprule
    \cmidrule[0.4pt](l{0.125em}){1-1}%
    \cmidrule[0.4pt](lc{0.125em}){2-2}%
    \multirow{3}{*}{\makecell{True Input 1 }}                   
    & \small\textnormal{\textit{P}: A group of people are gathered together.} \\
    & \small\textbf{\textit{H}: There is a group here.}\\
    & \textit{Label}: Entailment
    \\%\\
    \multirow{2}{*}{\makecell{Adversary 1}}
    & \small\textbf{\textit{H'}: There is a group \textcolor{red}{there}.}\\
    & \small\textnormal{\textit{Label}}: Contradiction
    \\\\
    \multirow{3}{*}{\makecell{True Input 2 }}                   
    & \small\textnormal{\textit{P}: A female lacrosse player jumps up.} \\
    & \small\textbf{\textit{H}: A football player sleeps.} \\
    & \textit{Label}: Contradiction
    \\%\\
    \multirow{2}{*}{\makecell{Adversary 2}}
    & \small\textbf{\textit{H'}: A football player \textcolor{red}{sits}.}\\
    & \textit{Label}: Neutral
    \\\\
    \multirow{3}{*}{\makecell{True Input 3 }}                   
    & \small\textnormal{\textit{P}: A man stands in a curvy corridor.} \\
    & \small\textbf{\textit{H'}: A man runs down a back alley.} \\
    & \textit{Label}: Contradiction
    \\%\\
    \multirow{2}{*}{\makecell{Adversary 3}}
    & \small\textbf{\textit{H'}: A man runs down a \textcolor{red}{ladder} alley.}\\
    & \small\textbf{\textit{Label}}: Neutral
    \\
    \bottomrule
    \end{tabular}
\end{sc}
\end{small}
%\end{center}
\vskip -0.15in
\end{table}
}
\noindent\textbf{Attack Success Rate (ASR).} We attack an SNLI classifier that has a test accuracy of 89.42\%. Given a pair (\textit{P, H}) with label $l$, its perturbed version (\textit{P, H'}) is adversarial if the classifier assigns the label $l$ to (\textit{P, H}), (\textit{P, H'}) is manually found to retain the label of (\textit{P, H}), and such label differs from the one the classifier assigns to (\textit{P, H'}).

Unlike for adversarial images, in order to compute the ASR for our text adversaries, we rely on human evaluation. The reason is that the sentence pair (\textit{P, H'}) we adversarially generate \textit{might not be adversarial to a human} since the new class the target model assigns to (\textit{P, H'}) may actually reflect the true relationship between \textit{P} and \textit{H'}. Consequently, we run a pilot study which we detail in Section 7.3.

\noindent\textbf{Pilot Study II - SNLI.} Using the transpose CNN as decoder $p_\phi$, we generate adversarial hypotheses for the SNLI sentence pairs with the premises kept unchanged. Then, we manually select 100 pairs of clean sentences (premise, hypothesis), and adversarial hypotheses. We also pick 100 pairs of sentences and adversarial hypotheses generated using~\cite{zhao2018generating}'s method against their treeLSTM classifier. We choose this classifier as its accuracy (89.04\%) is close to ours (89.42\%). Finally, to quantify the percentages of coherent text adversaries we generate, we randomly pick 100 pairs of sentences, and 100 pairs of sentences generated using ~\cite{zhao2018generating}'s treeLSTM to carry out a pilot study where we ask three questions (Q1) \textit{are the adversarial samples semantically sound?}, (Q2) \textit{are they similar to the true inputs?} and (Q3) \textit{what is the percentage of examples that are adversarial and semantically sound out of the random samples we select?} We report the evaluation results in Table~\ref{tab:p_study_snli}.
\begin{table}[ht]
\caption{Pilot Study II. Manual evaluation results for SNLI.}
\label{tab:p_study_snli}
\centering
\begin{small}
\begin{sc}
    \begin{tabular}{
        >{\arraybackslash}m{1.6cm}|
        >{\centering\arraybackslash}m{2.2cm}|
        >{\centering\arraybackslash}m{3.0cm}}
    \toprule
    Questions
    & 
    \specialcell[t]{Our Method} 
    & 
    \cite{zhao2018generating} 
    \\

    \cmidrule[0.4pt](lc{0.125em}){1-1}%
    \cmidrule[0.4pt](lc{0.125em}){2-2}%
    \cmidrule[0.4pt](lc{0.125em}){3-3}%

    Q1: Yes
    & 82.9 \% & 78.8 \% %$^\dagger$
    \\
    Q2: Yes
    & 61.2 \% & 55.9 \% 
    \\
    Q3 (pct.)
    & 60.3 \%  & 53.7 \%
    \\
    \bottomrule
    \end{tabular}
\end{sc}
\end{small}
\end{table}

\subsection{Evaluation against Defenses}~\label{sec:defenses}

We study the semantic soundness of the adversarial examples produced by our attack by attacking various defenses. For MNIST, we pick 100 images (10 for each digit) and generate adversarial examples against a 40-step PGD ResNet (M1) with $\epsilon_\text{attack}\leq 0.3$. We also target the certified defenses of~\cite{DBLP:journals/corr/abs-1801-09344} (M2) and~\cite{DBLP:journals/corr/abs-1711-00851} (M3) with $\epsilon_\text{attack}=0.1$. We repeat this study for the SVHN and CelebA datasets (for gender classification) by attacking a 40-step PGD ResNet. For all three datasets, we hand the images and the questionnaire (Q1, Q2, Q3) to 10 human subjects for manual evaluation. We report the results for MNIST in Table~\ref{tab:p_study_mnist}, and the results for CelebA and SVHN in Table~\ref{tab:p_study_celeba}. Our results show that our attack can produce semantics preserving adversarial examples with a high success rate against various defenses as well as different target datasets.

\begin{table}[ht]
\caption{Pilot Study I. Manual evaluation results of our attacks against M1 (40-step PGD), M2~(\cite{DBLP:journals/corr/abs-1801-09344}) and M3 (\cite{DBLP:journals/corr/abs-1711-00851}).}
\label{tab:p_study_mnist}
\centering
\begin{small}
\begin{sc}
    \begin{tabular}{
        >{\arraybackslash}m{1.6cm}|
        >{\centering\arraybackslash}m{1.6cm}|
        >{\centering\arraybackslash}m{1.6cm}|
        >{\centering\arraybackslash}m{1.6cm}}
    \toprule
    \multirow{3}{*}{Questions}
    & \multicolumn{3}{c}{MNIST}\\
    \cmidrule[0.4pt](lc{0.125em}){2-4}%
    & M1%\specialcell[t]{40-step PGD}
    & M2%\cite{DBLP:journals/corr/abs-1801-09344}  
    & M3%\cite{DBLP:journals/corr/abs-1711-00851}
    \\ %& SNLI \\ % end header
    \cmidrule[0.4pt](lc{0.125em}){1-1}%
    \cmidrule[0.4pt](lc{0.125em}){2-2}%
    \cmidrule[0.4pt](lc{0.125em}){3-3}%
    \cmidrule[0.4pt](lc{0.15em}){4-4}%

    Q1: Yes
    & 100 \%
    & 100 \%
    & 100 \%
    \\
    Q2: Yes
    & 100 \%
    & 100 \%
    & 100 \%
    \\
    Q3: No
    & 100 \%
    & 100 \%
    & 100 \%
    \\
    \bottomrule
    \end{tabular}
\end{sc}
\end{small}
\vskip -0.1in
\end{table}

\begin{table}[ht]
\caption{Pilot Study I. Our results for CelebA and SVHN.}
\label{tab:p_study_celeba}
\centering
\begin{small}
\begin{sc}
    \begin{tabular}{
        >{\arraybackslash}m{1.6cm}|
        >{\centering\arraybackslash}m{2.6cm}|
        >{\centering\arraybackslash}m{2.6cm}}
    \toprule
    Questions
    & 
    CelebA 
    & 
    SVHN 
    \\

    \cmidrule[0.4pt](lc{0.125em}){1-1}%
    \cmidrule[0.4pt](lc{0.125em}){2-2}%
    \cmidrule[0.4pt](lc{0.125em}){3-3}%

    Q1: Yes
    & 100 \% & 94.3 \%
    \\
    Q2: Yes
    & 100 \% &  96.8 \%
    \\
    Q3: No
    & 100 \% & 100 \%
    \\
    \bottomrule
    \end{tabular}
\end{sc}
\end{small}
%\vskip -0.1in
\end{table}

% \begin{definition} Let ($\mathcal{X}, d$) be a metric space and $h\colon\mathcal{X}\to\mathcal{X}$ a homeomorphism. For any point $u\in\mathcal{X}$, a neighborhood $\mathcal{U}$ of $u$ is \textit{invariant} under $h$ if: $v\in\mathcal{U}\Rightarrow h(v)\in\mathcal{U}$~\cite{10.1088/2053-2571/ab0281ch6}.
% \label{def:invariance}
% \end{definition}

\section{Posterior Formulation}~\label{sec:posterior} Similar to~\cite{DBLP:journals/corr/abs-1806-03836}, we formalize  $p(\theta|\mathcal{D})$ for every $\theta\in\Theta$ as:
\begin{equation*}
    \begin{split}
        p(\theta|\mathcal{D}) \propto p(\mathcal{D}|\theta) p(\theta) &= \prod\limits_{(x, \tilde{z})} p(\tilde{z}|x; \theta) p(\theta) \text{ where } x\in\mathcal{D} \text{ and } \tilde{z} \text{ is generated using Algorithm~\ref{alg:inversion} }\\
        &= \prod\limits_{(x, \tilde{z})} \mathcal{N}(\tilde{z}|f_{W}(x), \gamma^{-1}) %\prod\limits_{w\in W}
        \mathcal{N}(W|f_\eta(\xi), \lambda^{-1})\text{Gamma}(\gamma|a, b)
        \text{Gamma}(\lambda|a', b').
    \end{split}
\end{equation*}
Note that $\theta$ consists in fact of network parameters $W\sim f_\eta$ and scaling parameters $\gamma$ and $\lambda$. For notational simplicity, we used before the shorthands $\theta\sim f_{\eta}$. The parameters $\gamma$ and $\lambda$ are initially sampled from a Gamma distribution and updated as part of the training. In our experiments, we set the hyper-parameters of the Gamma distributions $a$ and $b$ to $1.0$ and $0.1$, and $a'$ and $b'$ to $1.0$. 

% \section{Manifold Alignment.}\label{sec:train} 
% Although GBSM confers us latent noise imperceptibility and sampling speed, $\Theta'$ may deviate from $\Theta$; in which case the manifolds they learn will mis-align. 
% To mitigate this issue, we regularize each $\theta'_m\in\Theta'$ after every GBSM update. In essence, we apply one SVGD update on $\Theta'$ to ensure that $\Theta'$ follows the transform maps constructed by the particles $\Theta$~\cite{junhan2017}.
% \begin{equation}
%     \begin{gathered}
%         \theta'_{t+1} \leftarrow \theta'_{t} + \alpha_{t}\pi(\theta'_t)\ \text{where}\\
%         \begin{aligned}
%              \pi(\theta'_t) = \frac{1}{M}\sum_{m=1}^M \Big[ & k(\theta'_t, \theta^m_t) \nabla_{\theta^m_t} \log p(\theta^m_t)  +  \nabla_{\theta^m_t} k(\theta'_t, \theta^m_t) \Big]
%         \label{eq:ta_prime_upd}
%         \end{aligned}
%     \end{gathered}
% \end{equation}
% We use the notation SVGD$_{\pi}(\Theta')$ to refer to the gradient update rule in Equation~\ref{eq:ta_prime_upd}. In this rule, the model instances $\Theta'$ determine their own update direction by consulting only the particles $\Theta$ instead of consulting each other. 

\section{$\ell_2$-norm an Upper Bound of $\ell_{\infty}$-norm}~\label{app:proof}
Given $x = (x_1, ..., x_n)\in \mathbb{R}^n$, $\|x\|_\infty = \max_i |x_i|$ and $\|x\|_2 = \sqrt{\sum_{i=1}^n x_i^2}$. If we let $|x_j|\coloneqq\max_i |x_i|$, given that $|x_j|^2 = x_j^2 \leq \sum_{i=1}^n x_i^2$, it follows that $\|x\|_\infty \leq \|x\|_2$. Hence, if $\|x\|_2 \leq \epsilon_{\text{attack}}$, then we have $\|x\|_\infty\leq  \epsilon_{\text{attack}}$. 

\section{Discussion}~\label{app:discussion} Here, we discuss the choices pertaining to the design of our approach and their limitations. \\

\textbf{Recognition Network.} As noted in~\cite{2015arXiv150505770J}, the Gaussian prior assumption in VAEs is too restrictive to generate meaningful enough latent codes~\cite{DBLP:journals/corr/ZhaoSE17b}. Thus, to produce informative latent codes, we use SVGD to learn the parameters of the encoder $E$. SVGD maintains a set of $M$ model instances. As an ensemble method, SVGD inherits the shortcomings of ensemble models most notably in space/time complexity for large $M$. Thus, instead of maintaining $2*M$ model instances, we maintain only one recognition network $f_\eta$ which learns to mimic the sampling dynamics of SVGD although it diverges a bit sometimes. \\

\textbf{Latent Noise Level.} The changes to the original inputs we perturb are captured by our reconstruction loss --- bounded by $\epsilon_\text{attack}$ (see Equation~\ref{eq:training}) --- which measures the imperceptibility of our adversarial perturbations in the input space. To get a sense of the amount of latent noise we inject to the clean codes $z_1, ..., z_M$, we compute the marginals of the clean and perturbed latent codes. As shown in Figure~\ref{fig:distribs}, the marginal distributions overlap relatively well. This means that the latent noise level is actually small.

\begin{figure}[ht]
\vskip -0.25in
\begin{center}
    \subfloat[MNIST]{{\includegraphics[width=3.3cm]{plots/mnist/no-kde6.png}}}
    \subfloat[CelebA]{{\includegraphics[width=3.3cm]{plots/celeba/no-kde14.png}}}
    \subfloat[SVHN]{{\includegraphics[width=3.3cm]{plots/svhn/plot.png}}}
    \subfloat[SNLI]{{\includegraphics[width=3.3cm]{plots/snli_1/no-kde19.png}}}
    \caption{Marginal distributions of clean (blue) and perturbed (red) latent codes over few minibatches.
    }
\label{fig:distribs}
\end{center}
\end{figure}
\label{discussion}

\textbf{Semantics Preservation (Text).} To construct adversarial text, we experiment with three architecture designs for the decoder $p_\phi$: (i.) a transpose CNN, (ii.) a language model, and (iii.) the decoder of a pre-trained ARAE model~\cite{pmlr-v80-zhao18b}. The transpose CNN generates more legible text than the other two designs although we notice sometimes some changes in meaning in the generated adversarial examples. Similar to~\cite{zhao2018generating}, a sizeable number of the examples we generate are not adversarial (see Table~\ref{tab:non_adv_snli_results_appendix} for some examples). 
Adversarial text generation is challenging in that small perturbations in the latent codes can go unnoticed at generation whereas high noise levels can render the outputs nonsensical. To produce adversarial sentences that faithfully preserve the meaning of the inputs, we need good sentence generators, like GPT~\cite{Radford2018ImprovingLU}, trained on large corpora. In our experiments, we consider only a vocabulary of size 10,000 words and sentences of length no more than 10 words to align our evaluation with the experimental choices of~\cite{zhao2018generating}.

%%%%%%%%%
\clearpage
\section{Adversarial Examples}~\label{app:adversarial_examples}
\subsection{Adversarial Images: CelebA}
Here, we provide few random samples of non-targeted adversarial examples we generate with our approach on the CelebA dataset as well as the clean reconstructions.
\begin{table*}[!thb]
\caption{CelebA samples, their clean reconstructions, and adversarial examples.}
\label{tab:results_celeba}
%\vskip -0.15in
\begin{center}
\begin{small}
\begin{sc}
    \begin{tabular}{
        >{\centering\arraybackslash}m{1.8cm}
        >{\centering\arraybackslash}m{6.5cm}
        >{\centering\arraybackslash}m{6.5cm}}
    \toprule
    % &
    % True inputs  
    % & 
    % Adversarial Examples 
    % \\
    % \cmidrule[0.4pt](lc{0.125em}){1-1}%
    % \cmidrule[0.4pt](lc{0.125em}){2-2}%  
    % \cmidrule[0.4pt](lc{0.125em}){3-3}% 
    Inputs 
    & 
    \includegraphics[width=0.35\textwidth, height=55mm]{samples/celeba/appendix/originals/original-18.jpg}
    & \includegraphics[width=0.35\textwidth, height=55mm]{samples/celeba/appendix/originals/original-19.jpg} 
    \\\cmidrule[0.4pt](lc{0.125em}){1-1}%
    Clean Reconstructions                   & 
    \includegraphics[width=0.35\textwidth, height=55mm]{samples/celeba/appendix/reconstructs/reconstruct-18.jpg}
    & \includegraphics[width=0.35\textwidth, height=55mm]{samples/celeba/appendix/reconstructs/reconstruct-19.jpg} 
    \\\cmidrule[0.4pt](lc{0.125em}){1-1}% 
    Adversarial Examples                     & 
    \includegraphics[width=0.35\textwidth, height=55mm]{samples/celeba/appendix/asr_reconstructs/adversaries-18.jpg}
    & \includegraphics[width=0.35\textwidth, height=55mm]{samples/celeba/appendix/asr_reconstructs/adversaries-19.jpg}
    \\
    \bottomrule
    \end{tabular}
\end{sc}
\end{small}
\end{center}
\vskip -0.1in
\end{table*}

\clearpage
\subsection{Adversarial Images: SVHN}
Here, we provide few random samples of non-targeted adversarial examples we generate with our approach on the SVHN dataset as well as the clean reconstructions.

\begin{table*}[!thb]
\caption{SVHN. Images  in red boxes are all adversarial.}
\label{tab:results_svhn}
%\vskip -0.15in
\begin{center}
\begin{small}
\begin{sc}
    \begin{tabular}{
        >{\centering\arraybackslash}m{1.8cm}
        >{\centering\arraybackslash}m{6.5cm}
        >{\centering\arraybackslash}m{6.5cm}}
    \toprule
    Inputs 
    & 
    \includegraphics[width=0.35\textwidth, height=55mm]{samples/svhn/appendix/originals-360.jpg}
    & \includegraphics[width=0.35\textwidth, height=55mm]{samples/svhn/appendix/originals-363.jpg}
    \\\cmidrule[0.4pt](lc{0.125em}){1-1}% 
    Clean Reconstructions                   & 
    \includegraphics[width=0.35\textwidth, height=55mm]{samples/svhn/appendix/reconstruct-360.jpg}
    & \includegraphics[width=0.35\textwidth, height=55mm]{samples/svhn/appendix/reconstruct-363.jpg} 
    \\\cmidrule[0.4pt](lc{0.125em}){1-1}% 
    Adversarial Examples                     & 
    \setlength{\fboxsep}{0pt}\fcolorbox{red}{black}{\fbox{\includegraphics[width=0.35\textwidth, height=55mm]{samples/svhn/appendix/adversaries-360.jpg}}}
    & \setlength{\fboxsep}{0pt}\fcolorbox{red}{black}{\fbox{\includegraphics[width=0.35\textwidth, height=55mm]{samples/svhn/appendix/adversaries-363.jpg}}}
    \\
    \bottomrule
    \end{tabular}
\end{sc}
\end{small}
\end{center}
%\vskip -0.1in
\end{table*}

\clearpage
\subsection{Adversarial Images: MNIST}
Here, we provide few random samples of non-targeted adversarial examples we generate with our approach on the MNIST dataset as well as the clean reconstructions. Both the reconstructed and the adversarial images look realistic and semantically correct although we notice some artifacts on the latter. Basic Iterative Methods~\cite{DBLP:journals/corr/KurakinGB16}, among other adversarial attacks, also suffer from this. Note that, however, in our case the marginal distributions of the latent codes of the inputs and their perturbed versions overlap quite well as illustrated in Figure~\ref{fig:distribs}. 

\begin{table*}[!thb]
\caption{MNIST. Images in red boxes are all adversarial.}
\label{tab:results_mnist}
%\vskip -0.15in
\centering
\begin{small}
\begin{sc}
    \begin{tabular}{
        >{\centering\arraybackslash}m{1.8cm}
        >{\centering\arraybackslash}m{6.5cm}
        >{\centering\arraybackslash}m{6.5cm}}
    \toprule
    Inputs                  
    & 
    \includegraphics[width=0.35\textwidth, height=55mm]{samples/mnist/appendix/originals-400-0.jpg}
    & 
    \includegraphics[width=0.35\textwidth, height=55mm]{samples/mnist/appendix/originals-400-200.jpg}
    \\\cmidrule[0.36pt](lc{0.125em}){1-1}% 
    Clean Reconstruction                   
    & 
    \includegraphics[width=0.35\textwidth, height=55mm]{samples/mnist/appendix/reconstruct-400-0.jpg}
    & 
    \includegraphics[width=0.35\textwidth, height=55mm]{samples/mnist/appendix/reconstruct-400-200.jpg} 
    \\\cmidrule[0.4pt](lc{0.125em}){1-1}% 
    Adversarial Examples                     
    & 
    \setlength{\fboxsep}{0pt}\fcolorbox{red}{black}{\fbox{\includegraphics[width=0.35\textwidth, height=55mm]{samples/mnist/appendix/adversaries-400-0.jpg}}}
    & 
    \setlength{\fboxsep}{0pt}\fcolorbox{red}{black}{\fbox{\includegraphics[width=0.35\textwidth, height=55mm]{samples/mnist/appendix/adversaries-400-200.jpg}}}
    \\
    \bottomrule
    \end{tabular}
\end{sc}
\end{small}
%\vskip -0.1in
\end{table*}

%\clearpage
%\label{page:adv_text}
\subsection{Adversarial Text: SNLI}
%Here, we provide few random samples of non-targeted adversarial examples we generate with our approach on the SNLI dataset.

\begin{table*}[htb]
\caption{Examples of adversarially generated hypotheses with the true premises kept unchanged.}
\label{tab:snli_results_appendix}
%\vskip -0.5in
\centering
\begin{small}
\begin{sc}
    \begin{tabular}{
        >{\arraybackslash}m{2.5cm}
        >{\arraybackslash}m{10.5cm}}
    \toprule
    \cmidrule[0.4pt](l{0.125em}){1-1}%
    \cmidrule[0.4pt](lc{0.125em}){2-2}%
    \\
    \multirow{3}{*}{\makecell{True Input 1 }}                   
    & \textnormal{\textit{P}: A white dog is running through the snow.}  \\
    & \textbf{\textit{H}: A cat stalking through the snow.} \\ 
    & \textit{Label}: Contradiction
    \\%\\
    \multirow{1}{*}{\makecell{Adversary}}
    & \textbf{\textit{H'}: A cat \textcolor{red}{hops in} the snow.} \textnormal{\textit{Label}}: Neutral
    \\
    \\\hline
    \\
    \multirow{3}{*}{\makecell{True Input 2 }}                   
    & \textnormal{\textit{P}: Three dogs are searching for something outside.} \\
    & \textbf{\textit{H}: There are four dogs.} \\
    & \textit{Label}: Contradiction
    \\%\\
    \multirow{1}{*}{\makecell{Adversary}}
    & \textbf{\textit{H'}: There are \textcolor{red}{five} dogs.} \textit{Label}: Neutral
    \\
    \\\hline
    \\
    \multirow{2}{*}{\makecell{True Input 3 }}                   
    & \textnormal{\textit{P}: A man waterskis while attached to a parachute.} \\ 
    & \textbf{\textit{H}: A bulldozer knocks down a house.} \\
    & \textit{Label}: Contradiction
    \\%\\
    \multirow{1}{*}{\makecell{Adversary}}
    & \textbf{\textit{H'}: A bulldozer knocks down a \textcolor{red}{cage}.} \small\textbf{\textit{Label}}: Entailment
    \\
    \\\hline
    \\
    \multirow{3}{*}{\makecell{True Input 4 }}                   
    & \textnormal{\textit{P}: A little girl playing with flowers.} \\ 
    & \textbf{\textit{H}: A little girl playing with a ball.} \\
    & \textit{Label}: Contradiction
    \\%\\
    \multirow{1}{*}{\makecell{Adversary}}
    & \textbf{\textit{H'}: A little girl \textcolor{red}{running} with a ball.} \textbf{\textit{Label}}: Neutral
    \\
    \\\hline
    \\
    \multirow{3}{*}{\makecell{True Input 5 }}                   
    & \textnormal{\textit{P}: People stand in front of a chalkboard.} \\ 
    & \textbf{\textit{H}: People stand outside a photography store.} \\ 
    & \textit{Label}: Contradiction
    \\%\\
    \multirow{1}{*}{\makecell{Adversary}}
    & \textbf{\textit{H'}: People stand \textcolor{red}{in front of a workshop}.} \textbf{\textit{Label}}: Neutral
    \\
    \\\hline
    \\
    \multirow{3}{*}{\makecell{True Input 6 }}                   
    & \textnormal{\textit{P}: Musician entertaining \textbf{his} audience.} \\ 
    & \textbf{\textit{H}: The woman played the trumpet.} \\
    & \textit{Label}: Contradiction
    \\%\\
    \multirow{2}{*}{\makecell{Adversary}}
    & \textbf{\textit{H'}: The woman played the \textcolor{red}{drums}.} \textbf{\textit{Label}}: Entailment
    \\
    \\\hline
    \\
    \multirow{3}{*}{\makecell{True Input 7 }}                   
    & \textnormal{\textit{P}: A kid on a slip and slide.} \\ 
    & \textbf{\textit{H}: A small child is \textcolor{red}{inside} eating their dinner.} \\
    & \textit{Label}: Contradiction
    \\%\\
    \multirow{1}{*}{\makecell{Adversary}}
    & \textbf{\textit{H'}: A small child is eating their dinner.} \textbf{\textit{Label}}: Entailment
    \\
    \\\hline
    \\
    \multirow{3}{*}{\makecell{True Input 8 }}                   
    & \textnormal{\textit{P}:  A deer jumping over a fence.} \\ 
    & \textbf{\textit{H}: A deer laying in the grass.} \textit{Label}: Contradiction
    \\%\\
    \multirow{2}{*}{\makecell{Adversary}}
    & \textbf{\textit{H'}: A \textcolor{red}{pony} laying in the grass.}\\& \textbf{\textit{Label}}: Entailment
    \\
    \\\hline
    \\
    \multirow{3}{*}{\makecell{True Input 9 }}                   
    & \textnormal{\textit{P}: Two vendors are on a curb selling balloons.} \\ 
    & \textbf{\textit{H}: Three people sell lemonade by the road side.} \\&
    \textit{Label}: Contradiction
    \\%\\
    \multirow{2}{*}{\makecell{Adversary}}
    & \textbf{\textit{H'}: Three people sell \textcolor{red}{artwork} by the road side.}\\& \textbf{\textit{Label}}: Entailment
    \\
    \\
    \bottomrule
    \end{tabular}
\end{sc}
\end{small}
\end{table*}

\clearpage

\begin{table*}[!htb]
\caption{Misses. Some generated examples deemed adversarial by our method that are not.}
\label{tab:non_adv_snli_results_appendix}
%\vskip -0.5in
\centering
\begin{small}
\begin{sc}
    \begin{tabular}{
        >{\arraybackslash}m{2.5cm}
        >{\arraybackslash}m{10.5cm}}
    \toprule
    \cmidrule[0.4pt](l{0.125em}){1-1}%
    \cmidrule[0.4pt](lc{0.125em}){2-2}%
    \\
    \multirow{3}{*}{\makecell{True Input 1 }}                   
    & \textnormal{\textit{P}: A man is operating some type of a vessel.}  \\
    & \textbf{\textit{H}: A dog in kennel.} \\ 
    & \textit{Label}: Contradiction
    \\%\\
    \multirow{1}{*}{\makecell{Generated}}
    & \textbf{\textit{H'}: A dog in \textcolor{red}{disguise}.} \textnormal{\textit{Label}}: Contradiction
    \\
    \\\hline
    \\
    \multirow{3}{*}{\makecell{True Input 2 }}                   
    & \textnormal{\textit{P}: A skier.} \\
    & \textbf{\textit{H}: Someone is skiing.} \\
    & \textit{Label}: Entailment
    \\%\\
    \multirow{1}{*}{\makecell{Generated}}
    & \textbf{\textit{H'}: \textcolor{red}{Man} is skiing.} \textit{Label}: Neutral
    \\
    \\\hline
    \\
    \multirow{2}{*}{\makecell{True Input 3 }}                   
    & \textnormal{\textit{P}: This is a bustling city street.} \\ 
    & \textbf{\textit{H}: There are a lot of people walking along.} \\
    & \textit{Label}: Entailment
    \\%\\
    \multirow{1}{*}{\makecell{Generated}}
    & \textbf{\textit{H'}: There are a lot \textcolor{red}{girls} walking along.} \small\textbf{\textit{Label}}: Neutral
    \\
    \\\hline
    \\
    \multirow{3}{*}{\makecell{True Input 4 }}                   
    & \textnormal{\textit{P}: A soldier is looking out of a window.} \\ 
    & \textbf{\textit{H}: The prisoner's cell is windowless.} \\
    & \textit{Label}: Contradiction
    \\%\\
    \multirow{1}{*}{\makecell{Generated}}
    & \textbf{\textit{H'}: The prisoner's \textcolor{red}{home} is windowless.} \textbf{\textit{Label}}: Contradiction
    \\
    \\\hline
    \\
    \multirow{3}{*}{\makecell{True Input 5 }}                   
    & \textnormal{\textit{P}: Four people sitting on a low cement ledge.} \\ 
    & \textbf{\textit{H}: There are four people.} \\ 
    & \textit{Label}: Entailment
    \\%\\
    \multirow{1}{*}{\makecell{Generated}}
    & \textbf{\textit{H'}: There are \textcolor{red}{several} people.} \textbf{\textit{Label}}: Neutral
    \\
    \\\hline
    \\
    \multirow{3}{*}{\makecell{True Input 6 }}                   
    & \textnormal{\textit{P}: Three youngsters shovel a huge pile of snow.} \\ 
    & \textbf{\textit{H}: Children working to clear snow.} \\
    & \textit{Label}: Entailment
    \\%\\
    \multirow{2}{*}{\makecell{Generated}}
    & \textbf{\textit{H'}: \textcolor{red}{Kids} working to clear snow.} \textbf{\textit{Label}}: Neutral
    \\
    \\\hline
    \\
    \multirow{3}{*}{\makecell{True Input 7 }}                   
    & \textnormal{\textit{P}: Boys at an amphitheater.} \\ 
    & \textbf{\textit{H}: Boys at a show.} \\
    & \textit{Label}: Entailment
    \\%\\
    \multirow{1}{*}{\makecell{Generated}}
    & \textbf{\textit{H'}: Boys \textcolor{red}{in} a show.} \textbf{\textit{Label}}: Neutral
    \\
    \\\hline
    \\
    \multirow{3}{*}{\makecell{True Input 8 }}                   
    & \textnormal{\textit{P}: Male child holding a yellow balloon.} \\ 
    & \textbf{\textit{H}: Boy holding big balloon.} \textit{Label}: Neutral
    \\%\\
    \multirow{2}{*}{\makecell{Generated}}
    & \textbf{\textit{H'}: Boy holding \textcolor{red}{large} balloon.}\\& \textbf{\textit{Label}}: Neutral
    \\
    \\\hline
    \\
    \multirow{3}{*}{\makecell{True Input 9 }}                   
    & \textnormal{\textit{P}: Women in their swimsuits sunbathe on the sand.} \\ 
    & \textbf{\textit{H}: Women under the sun on the sand.} \\&
    \textit{Label}: Entailment
    \\%\\
    \multirow{2}{*}{\makecell{Generated}}
    & \textbf{\textit{H'}: \textcolor{red}{Family} under the sun on the sand.}\\& \textbf{\textit{Label}}: Neutral
    \\
    \\
    \bottomrule
    \end{tabular}
\end{sc}
\end{small}
\end{table*}

\clearpage

\section{Experimental Settings}
\begin{table*}[htb]
\caption{Model Configurations + SNLI Classifier + Hyper-parameters.}
\label{tab:configs}
\vskip 0.15in
\begin{center}
\begin{small}
\begin{sc}
    \begin{tabular}{
        >{\arraybackslash}m{4.0cm}|
        >{\arraybackslash}m{2.5cm}|
        >{\centering\arraybackslash}m{6.0cm}} %
    \toprule
    & Name
    & Configuration \\ % end header
    \cmidrule[0.4pt](ll{0.125em}){1-1}%
    \cmidrule[0.4pt](lc{0.125em}){2-2}%
    \cmidrule[0.4pt](lc{0.125em}){3-3}%
    \multirow{1}{*}{Recognition Networks}
    & $f_\eta$ 
    & \makecell{Input Dim: 50, \\Hidden Layers: [60, 70], \\Output Dim: Num weights \& biases in $\theta_m$} \\
    % \\\cline{2-3}\\ % end of sub-row 
    % & $f_\eta'$ 
    % & \makecell{Input Dim: 50, \\Hidden Layers: [60, 70], \\Output Dim: Num weights \& biases in $\theta'_m$} \\ % end of row
    
    \\ \hline\\
    
    \multirow{1}{*}{Model Instances} 
    & Particles $\theta_m$ 
    & \makecell{Input Dim: $28\times 28$ (MNIST), \\$64\times 64$ (CelebA), \\$32\times 32$ (SVHN), 300 (SNLI) \\
    Hidden Layers: [40, 40] \\ Output Dim (latent code): 100} \\
    % \\\cline{2-3}  \\
    % & Parameters $\theta'_m$ 
    % & \makecell{Input Dim:  $28\times 28$ (MNIST), \\$64\times 64$ (CelebA), \\$32\times 32$ (SVHN), 100 (SNLI) \\
    % Hidden Layers: [40, 40] \\ Output Dim (latent code): 100} \\
    
    \\ \hline\\
    
    Feature Extractor
    &
    \multicolumn{2}{c}{\makecell{Input Dim: $28\times28\times 1$ (MNIST), $64\times 64\times 3$ (CelebA), \\$32\times 32\times 3$ (SVHN), $10\times 100$ (SNLI) \\
    Hidden Layers: [40, 40] \\ Output Dim:  $28\times28$ (MNIST), $64\times 64$ (CelebA), \\$32\times 32$ (SVHN), $100$ (SNLI)}} \\
    
    \\ \hline \\
    
    \multirow{4}{*}{Decoder}
    & Transpose CNN
    & \makecell{For CelebA \& SVHN: [filters: 64, stride: 2, \\ kernel: 5]$\times$ 3\\ 
    For SNLI: [filters: 64, stride: 1, \\ kernel: 5]$\times$ 3}\\ 
    \\\cline{2-3}\\ % end of sub-row
    & Language Model 
    & \makecell{Vocabulary Size: 11,000 words\\
    Max Sentence Length: 10 words}\\ % end of row
    
    \\ \hline\hline \\

    \multirow{1}{*}{ SNLI classifier}
    & 
    \multicolumn{2}{c}{\makecell{Input Dim: 200, Hidden Layers: [100, 100, 100], Output Dim: 3}} 
    \\\\
    \midrule\\
    \multicolumn{1}{l|}{Learning Rates}&\multicolumn{2}{p{9cm}}{$\alpha=10^{-2} \text{ and } \beta=10^{-3}$}\\
    \\\hline\\
    \multicolumn{1}{l|}{More settings}&\multicolumn{2}{p{9.5cm}}{Batch size: 64, Inner-updates: 3, Training epochs: 1000, $M=5$}
    \\\\ 
    \bottomrule
    \end{tabular}
    \label{tab:architec}
\end{sc}
\end{small}
\end{center}
\end{table*}

\section{Related Work} ~\label{app:related}
\noindent\textbf{Manifold Learning.} VAEs are generally used to learn  manifolds~\cite{DBLP:journals/corr/abs-1808-06088,2018arXiv180704689F,higgins2016} by maximizing the ELBO of the data log-likelihood~\cite{DBLP:journals/corr/abs-1711-00464,2017arXiv170901846C}. Optimizing the ELBO entails reparameterizing the encoder to a Gaussian distribution~\cite{kingma2014}. This reparameterization is, however, restrictive~\cite{2015arXiv150505770J} as it may lead to learning poorly the manifold of the data~\cite{DBLP:journals/corr/ZhaoSE17b}. 
To alleviate this issue, we use SVGD. While our approach and \cite{yuchen2017} may look similar, we use Bayesian inference which is more principled than dropout~\cite{2017arXiv171102989H}. 
\vspace{.1em}

\noindent\textbf{Adversarial Examples.} Studies in adversarial deep learning~\cite{DBLP:journals/corr/abs-1802-00420,athalye2017,DBLP:journals/corr/KurakinGB16,ianj.goodfellow2014} can be categorized into two groups. The first group~\cite{athalye2017,DBLP:journals/corr/CarliniW16a,DBLP:journals/corr/Moosavi-Dezfooli16} proposes to generate adversarial examples directly in the input space of the source inputs by distorting, occluding or changing illumination in images to cause changes in classification. The second group~\cite{DBLP:conf/nips/SongSKE18,zhao2018generating}, where our work belongs, uses generative models to search for adversarial examples in the dense and continuous representations of the data rather than in its input space. 

\textit{Adversarial Images} 
\cite{DBLP:conf/nips/SongSKE18} propose to construct unrestricted adversarial examples by training a conditional GAN that constrains the search region for a latent code $z'$ in the neighborhood of a target $z$. \cite{zhao2018generating} use also a GAN to map input images to a latent space where they conduct their search for adversarial examples. To our knowledge, these studies are the closest to ours. Unlike in \cite{DBLP:conf/nips/SongSKE18,zhao2018generating}, however, our adversarial perturbations are learned. Moreover, we do not restrict the search for adversarial examples to uniformly-bounded regions. In contrast also to \cite{DBLP:conf/nips/SongSKE18} and \cite{zhao2018generating}, where the search for adversarial examples is iterative and decoupled from the training of the GANs, our method is end-to-end. Lastly, by capturing the uncertainty induced by embedding the data, we generate more realistic adversarial examples.

\textit{Adversarial Text:} 
Previous studies on adversarial text generation~\cite{pmlr-v80-zhao18b,DBLP:journals/corr/JiaL17,DBLP:journals/corr/Alvarez-MelisJ17,DBLP:journals/corr/LiMJ16a} perform word erasures and replacements directly in the input space using domain-specific rules or heuristics, or they require manual curation. Similar to us, \cite{zhao2018generating} propose to search for textual adversarial examples in the latent representation of the data. However, in addition to the differences aforementioned for images, the search for adversarial examples is handled in our case by an efficient gradient-based optimization method.
